# Supplementary material for: Compressibility measurement of the thermal MI--BG transition in an optical lattice
Source: arXiv:2506.16466 ancillary file (2025-06-19)
Supplement: Supplementary file 1 [file SupplementaryMaterial.pdf]

# Supplementary Material for "Compressibility measurement of the thermal MI–BG transition in an optical lattice"

Phil Russ,[1,*] Mi Yan,[2,†] Nicholas Kowalski,[1] Laura Wadleigh,[1,‡] Vito W. Scarola,[2] and Brian DeMarco[1,§]

[1]*Department of Physics, University of Illinois Urbana-Champaign, Urbana, Illinois 61801, USA*

[2]*Department of Physics, Virginia Tech, Blacksburg, Virginia 24061, USA*

(Dated: June 19, 2025)

# I. EXPERIMENTAL METHODS

## A. Experimental Sequence

Using standard techniques, a nearly pure BEC of $^{87}$Rb atoms is prepared in the $|1,-1\rangle$ hyperfine ground state in a crossed dipole-laser trap [1]. The lattice and disorder potentials are ramped on over 100 ms using an exponential ramp with a 200 ms time constant, resulting in an almost linear ramp. Following a static hold of all potentials for 2 ms, the lattice depth is ramped to 40 $E_R$ ($E_R = \frac{h^2}{2m\lambda_L^2}$ is the recoil energy of the lattice light, where $h$ is the Planck constant, $m$ is the atomic mass and $\lambda_L$ is the lattice wavelength) in 0.5 ms to halt all dynamics. A bias field of 3.3 G, used as a control switch for the spin exchange process, is ramped on over 5 ms. A pair of secondary magnetic fields are adjusted over a total duration of 50 ms in order to provide a small net residual field during the spin exchange process. Once the external fields are prepared, adiabatic rapid passage using an applied microwave-frequency magnetic field is performed in 5 ms to transfer the atoms to the $|2,-1\rangle$ hyperfine ground state. To initiate the spin exchange process, the bias field is ramped off in 0.1 ms, yielding a small residual magnetic field of 0.35 G. After a 1.8-2 ms hold time during which spin exchange occurs, a vertical magnetic field gradient is snapped on, and bandmapping is performed by ramping off the lattice potential in 0.2 ms. This magnetic field gradient serves the dual purpose of halting the spin exchange process and to spatially separate the spin states during time of flight. The time of flight duration is adjusted to achieve sufficiently low optical density (OD) and large gas separation. Finally, absorption imaging is performed and an OD image is generated.

## B. Spin Exchange

Spin exchange in the $F = 2$ hyperfine ground state [2, 3] is leveraged to detect the presence of double occupancies. Counting the number of atoms in the participating spin states allows for the simultaneous quantification of both the total atom number, $N$, and the fraction of atoms on doubly occupied sites, $D$. The spin dynamics are described by a

* Present address: Upgrade, San Francisco, California 94111, USA.
† Present address: Wolfram Research, Champaign, Illinois 61820, USA.
‡ Present address: Atom Computing, Boulder, Colorado 80301, USA.
§ Corresponding author: bdemarco@illinois.edu

two-level system with Rabi rate $\Omega$ and detuning $\delta$, where $\Omega$ and $\delta$ are determined by the matrix elements of the two-body interaction potential.

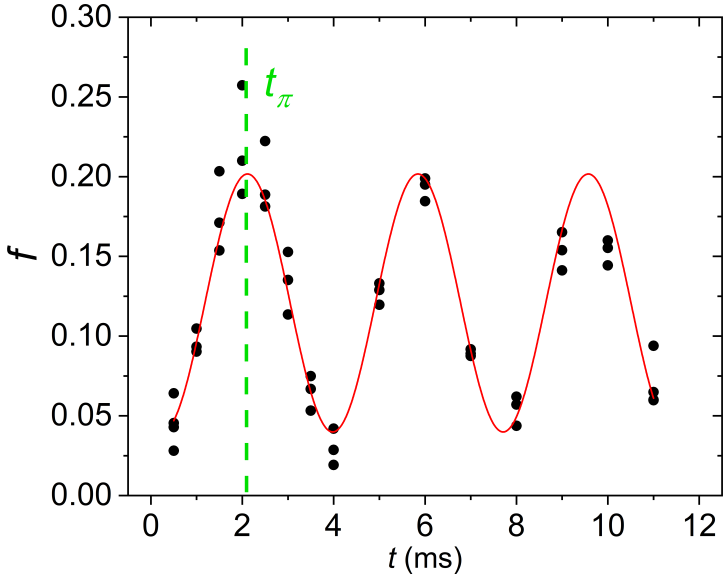


FIG. 1. A plot of the observed spin exchange oscillation for $N \approx 40000$ atoms, where $f$ is the fraction of atoms in $|2,-2\rangle \otimes |2,0\rangle$ for various hold times $t$ in the small magnetic field, and $t_\pi$ is the $\pi$-time of the spin exchange oscillation.

For atoms on sites with double occupancy, the initial state is $|2,-1\rangle \otimes |2,-1\rangle$ leaving $|2,-2\rangle \otimes |2,0\rangle$ as the only accessible final state due to conservation of total magnetization. The spin composition is allowed to evolve for one $\pi$-time of the spin exchange oscillation in low magnetic field after which double occupancies populate the final state. The small static field present during spin exchange means $\delta/\Omega \ll 1$, and the peak amplitude of the spin-exchange oscillation is approximately 97% of the on-resonance amplitude.

### C. Constraining Entropy and Trap Frequency

To infer the trap frequency $\omega$ and entropy-per-particle $S/N$, a prediction of the behavior of the fraction of atoms on doubly-occupied sites $D$ vs the total atom number $N$ is computed by simulating the system in the atomic limit (tunneling energy $t \to 0$) of the disordered Bose–Hubbard model (DBHM) for fixed values of $\omega$ and $S/N$. Measurements of $D$ vs $N$ are compared to these predictions in the atomic limit, and $\omega$ and $S/N$ are constrained using

least-squares minimization. This calculation is performed for a clean lattice $\Delta = 0$, while a calculation including disorder is presented in Section II D. To fully constrain both $S/N$ and $\omega$ requires predictions of at large atom number, which is computationally expensive and beyond the scope of this work when including disorder. Therefore, we make the approximation that the addition of disorder does not change $S/N$ or $\omega$. The inferred entropy and trap frequency are used to determine the atom number corresponding to unit filling, $N_1$, at which we measure the compressibility for finite $\Delta$.

Taking $t \to 0$ for the DBHM yields the atomic limit Hamiltonian,

$$\mathrm{H}^{\mathrm{A}} = \sum_i \left[ \frac{U}{2} \hat{n}_i (\hat{n}_i - 1) + (\epsilon_i + \Omega^2 r_i^2) \hat{n}_i \right], \tag{1}$$

where $\Omega^2 = m\omega^2/2$, $m$ is the atomic mass, $U$ is the interaction strength, and $\epsilon$ is the site occupation energy. Working in this limit is well justified since $t \ll k_B T \ll U$ in this experiment. The assumed adiabaticity of the lattice ramp as well as negligible atom loss motivates the use of $S/N$ instead of $T$ as the experimentally relevant thermal energy parameter. To generate predictions of $D$ vs $N$, $N$ and $D$ are found from $\mathrm{H}^{\mathrm{A}}$ under the assumption of fixed $\omega$ and $S/N$ by computing the average density and two-atom contribution to the density on each site and then summing over all lattice sites. This is done using statistical mechanics, where the equations for $N$, $D$ and $S/N$ in terms of $\mathcal{Z}_i$, the partition function on site $i$, are

$$\mathcal{Z}_i = \sum_{p=0}^{10} \mathrm{e}^{\beta p [\mu - \epsilon_i - \frac{U}{2}(p-1) - \Omega^2 r_i^2]} \tag{2}$$

$$N = \sum_i n_i = \sum_i \frac{1}{\mathcal{Z}_i} \sum_{p=1}^{10} p \mathrm{e}^{\beta p [\mu - \epsilon_i - \frac{U}{2}(p-1) - \Omega^2 r_i^2]} \tag{3}$$

$$D = \frac{2}{N} \sum_i d_i = \frac{2}{N} \sum_i \frac{\mathrm{e}^{-\beta[2(\epsilon_i + \Omega^2 r_i^2 - \mu) + U]}}{\mathcal{Z}_i} \tag{4}$$

$$S/N = \frac{1}{N} \sum_i s_i = \frac{k_B}{N} \sum_i \Big( \ln \mathcal{Z}_i - \frac{\beta}{\mathcal{Z}_i} \frac{\partial \mathcal{Z}_i}{\partial \beta} \Big), \tag{5}$$

where $\mu$ is the chemical potential, $\beta = (k_B T)^{-1}$ and the sum is performed over a truncated site occupation basis $p$. The truncation value ($n_{max} = 10$) is chosen to be much larger than the peak occupancy in the experiment. The sum over lattice sites is performed over a grid of positions in 3D space. The dimensions of this grid are chosen such that $n_i$ vanishes for sites

near the edge of the system as required by the presence of the external trapping potential. This is ensured by increasing the grid size until the computed $N$ and $S/N$ are constant.

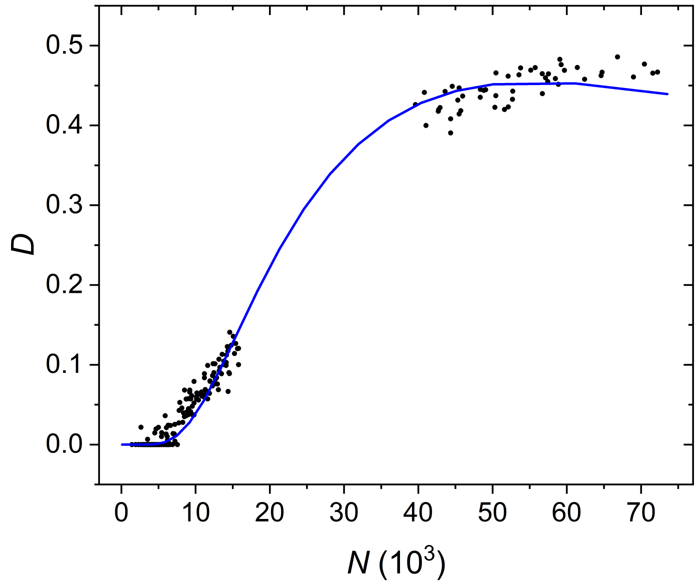


FIG. 2. A plot of measured $D$ vs $N$ at $s/E_R = 20$. The blue line is the prediction from the atomic limit for $\omega_{exp} = 109$ Hz and $S/N = 0.84k_B$.

The measured and predicted $D$ are compared for the clean case, $\Delta = 0$, in order to constrain $\omega$ and $S/N$. Curves of $D$ from the atomic limit for the range of $N$ in the experiment are produced at fixed $\omega$ and $S/N$. Using these curves to compare experiment and theory, the entropy-per-particle and overall trap frequency consistent with the experiment, $\omega_{exp}$ and $S/N_{exp}$, respectively, are determined through least-squares fitting. The sum of squared residuals $\chi(\omega, S/N) = \sum_{\mathcal{O}} [D_{\mathcal{O}} - \mathcal{D}_{\omega,S/N}(N_{\mathcal{O}})]^2$ is calculated where $\mathcal{O}$ is the set of observations, $D_{\mathcal{O}}$ is the measured double occupancy, and $\mathcal{D}_{S/N,\omega}$ is the prediction from the atomic limit at the measured atom number $N_{\mathcal{O}}$. Fitting $\chi$ near its minimum to an elliptic paraboloid, the best fit parameters for the vertex correspond to $\omega_{exp}$ and $S/N_{exp}$. Data from the experiment is only required in two regions in order to constrain $S/N_{exp}$ and $\omega_{exp}$ adequately: at low $N$ to capture the activation of $D$, and at large $N$ near the peak $D$. An example best-fit curve is shown in Figure 2. Having eliminated the free parameters, unit filling can be computed for $\Delta \geq 0$, since the distribution of $\epsilon$ for speckle disorder is known and $\Delta$ is calibrated in the experiment. The atom number corresponding to unit filling is $N_1 = N(\mu = \frac{U}{2} + \Delta)$ using

$\omega_{exp}$ and $S/N_{exp}$.

| $s$ ($E_R$) | $t/U$ | $S/N$ ($k_B$) | $\omega/2\pi$ (Hz) |
|---|---|---|---|
| 16 | 0.0124 | $0.7 \pm 0.1$ | $95.4 \pm 0.2$ |
| 20 | 0.0048 | $0.8 \pm 0.1$ | $108.7 \pm 0.2$ |
| 25 | 0.0017 | $0.7 \pm 0.1$ | $115.5 \pm 0.2$ |

TABLE I. Entropy per particle and trap frequency for each lattice depth, obtained by least-squares fitting predictions in the atomic limit to experimental data at $\Delta = 0$. Uncertainties represent uncertainty in fit parameters.

### D. Machine Learning Image Analysis

A two step technique was developed for analyzing images from the experiment in order to quantify $D$. First, least-squares fitting to a gaussian function is performed on the image of the $|2, -2\rangle$ and $|2, 0\rangle$ gases to serve as a discriminator for the presence of a gas. For each region, the gaussian widths, $s_{x,y}$, are compared to the respective gas width averages, $w_{x,y}$, determined from gaussian fits to high signal-to-noise gases in the experiment. For each region in each image, if simultaneously $|w_x - s_x| \leq 2$ and $|w_y - s_y| \leq 2$ (in units of pixels) it is considered to contain a gas, and the atom number is computed from the pixel sum. Otherwise, the region is passed to an image classifier generated using machine learning (ML) techniques which determines the probability of the region being empty, $P_e$. The value of $P_e$ is used to classify the region as empty or containing an atomic gas though comparison to a selected threshold probability, $P_{th}$. For $P_e \geq P_{th}$, the region is considered empty and the atom number is set to zero and for $P_e < P_{th}$, the region is considered to contain a gas, and the atom number is taken to be equal to the pixel sum result. Any images for which there is negative double occupancy after passing through the classifier are excluded.

Shown in Fig. 3 is a comparison of the measured $D$ with the pixel summing and two-step ML analysis techniques. As discussed in both the main text and in the theory methods (Section II), the double occupancy is predicted to be approximately zero at low atom number. Noise in the low atom number images obscures this behavior. The two-step ML analysis technique significantly increases the quality of the data. At small $N$ where $D$ is constant,

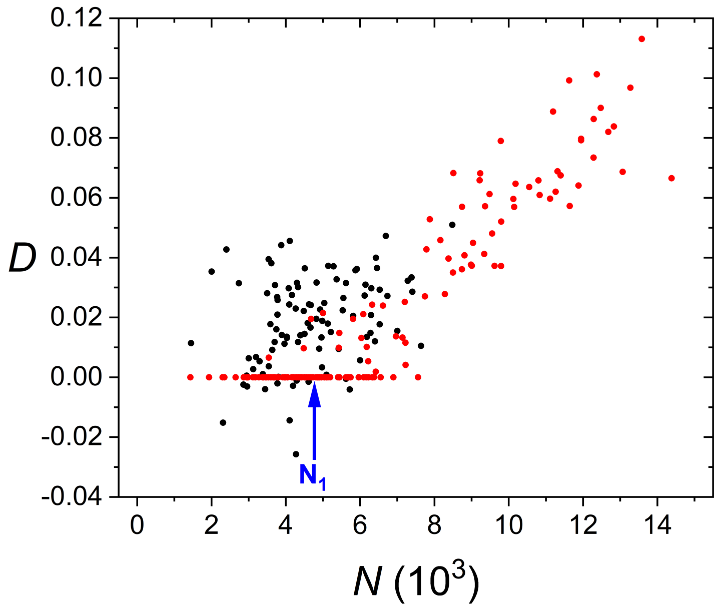


FIG. 3. Comparing image analysis methods for $s/E_R = 20$ at $\Delta/E_R = 0$. The red points are the result of applying the two-step ML analysis to the experimental images. The black points are the result of pixel summing. The blue arrow labels the total atom number corresponding to an average filling of one atom per site, $N_1$.

most of the points that have finite $D$ with pixel summing become zero, which is consistent with MI physics. As $D$ begins to increase, fewer and fewer of the pixel sum points are affected, until the two analysis methods agree consistently. Cases of negative double occupancy due to pixel summing are also greatly reduced. For instance, 75% of cases are eliminated in the $s/E_R = 20$ data set across all $\Delta$. The two-step technique accomplishes the difficult feat of improving double occupancy resolution in the experiment to the level of 0.01. Most importantly, the technique reduces the uncertainty in the measured compressibility. This is evident in Fig. 3 at the atom number corresponding to unit filling, $N_1$, on which the fitting window for extracting the compressibility is centered. Consequently, threshold behavior is exposed where the compressibility remains small for small $\Delta$ and increases for large $\Delta$. The reduced uncertainty in compressibility yields reduced uncertainty in the extracted threshold disorder for characterizing the onset of increasing compressibility.

The image classifier is generated using the **Classify** function in Wolfram Mathematica using the three options **Method**, **PerformanceGoal**, and **ValidationSet**. For the options **Method** and **PerformanceGoal**, "GradientBoostedTrees" and "Quality" are chosen, re-

spectively. Training images are generated artificially using models for the atomic gas as the signal and fluctuations in the background as the noise. The training set consists of 60,000 images, 5,000 containing a gas of atoms and 55,000 without. An additional 1,250 images containing a gas and 13,000 images without are used during training to combat overfitting using the option **ValidationSet**.

The density distribution of the atomic gas is modeled as having a Gaussian profile. Images from the experiment containing gases with high signal-to-noise are fit to a Gaussian function to determine the range of gas positions and widths. Artificial gases for training images are generated by specifying the atom number, position and widths for the Gaussian density profile. Analysis of pixel value histograms for empty images indicates the background noise has a Gaussian distribution. Artificial backgrounds are generated by specifying a mean and variance characteristic of empty images from the experiment and sampling the corresponding Gaussian distribution. A training image is obtained by superimposing one artificial background and one artificial gas of known atom number. Using real images is impractical due to the long time required to collect a set that sufficiently samples the relevant parameter space consisting of the atomic gas and background parameters, and the large amount of storage space they occupy. Another issue is the difficultly of determining the atom number in images, which is useful for training the classifier and characterizing its performance. This is especially important in the situation most relevant to this experiment, namely, when double occupancy is small, and hence the $|2,-2\rangle$ and $|2,0\rangle$ regions of the image have low signal-to-noise ratio.

The performance of the classifier is evaluated using test sets of 5000 artificial images containing gases of known, fixed atom number, $N_{test}$. For each image in a set, $P_e$ is obtained from the image classifier and shown in Fig. 4 is the $P_e$ distribution for the test sets obtained by binning the classifier output and finding the fraction of images in each bin. The probability threshold, $P_{th}$, for classifying an image as empty is determined based on the distribution of $P_e$ from the $N_{test} = 0$ set. To achieve significant reduction in the uncertainty of the calculated compressibility in the experiment, $P_{th}$ is chosen such that $P_e \geq P_{th}$ for 99.9% of images in the $N_{test} = 0$ set. A second plot for characterizing the classifier performance is shown in Fig. 5, called a receiver operating characteristic (ROC) curve. This was produced by passing an artificial test set to the classifier containing 2500 empty images and 2500 images containing gases of up to 1000 atoms. The cut off of 1000 atoms corresponds

to the largest gas the classifier encounters in the experimental data. The ROC curve gives the true positive rate $TPR = \frac{TP}{P}$ as a function of the false positive rate $FPR = \frac{FP}{N}$ for $P_{th}$ ranging from 0 to 1, where $TP$ and $FP$ are the number of true positives and false positives, respectively, identified by the classifier and $P$ and $N$ are the total number of positive and negative cases, respectively. The standard comparison is the performance relative to random guessing where the larger the separation of the classifier ROC above (below) the random guess result, the better (worse) the classifier performance. For the $P_{th} \approx 0.95$ in this work, $TPR \approx 0.999$ and $FPR \approx 0.14$. Finally, the precision/positive predictive value $PPV = \frac{TP}{TP+FP} \approx 0.88$ for $P_{th} \approx 0.95$.

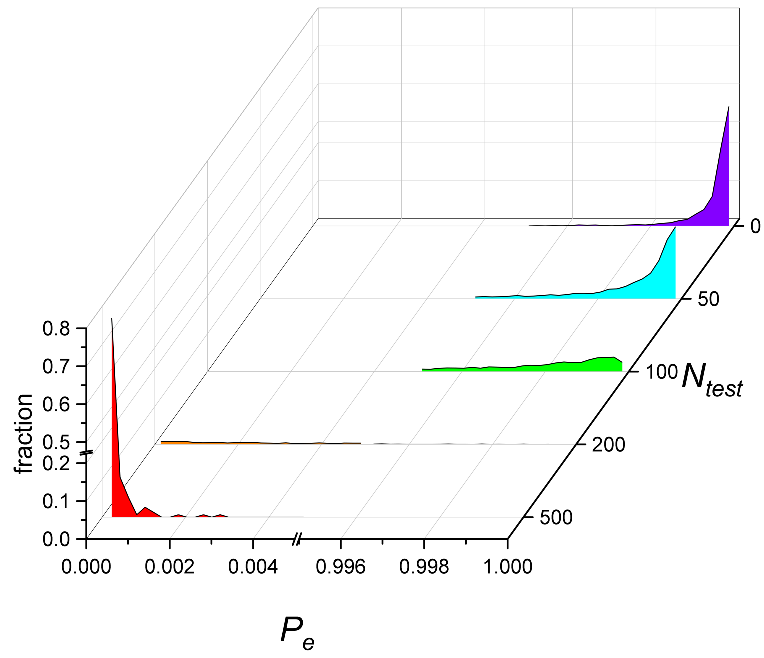


FIG. 4. Distribution of $P_e$ from image classifier for sets of 5000 artificial images containing a gas of $N_{test}$ atoms. The dashed purple line shows the chosen $P_{th}$.

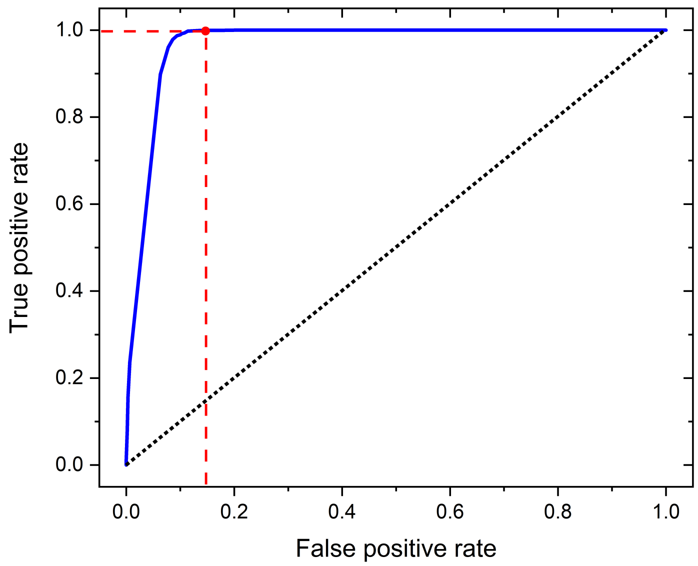


FIG. 5. The ROC curve for the image classifier plotted as the blue solid line. The red dot and dashed lines indicate $P_{th} \approx 0.95$. The black short dashed line gives the result for random guessing.

## II. THEORY METHODS

### A. Mean-field Limit

In this section, we discuss how we reduce the Bose-Hubbard model to a local mean field theory. The single-band Bose-Hubbard model is an excellent approximation to bosons in a deep optical lattice [4]:

$$H = -t \sum_{\langle i,j \rangle} (b_i^\dagger b_j + H.c.) + \frac{U}{2} \sum_i n_i (n_i - 1) - \sum_i \mu_i n_i. \tag{6}$$

Here, $b_i^\dagger$ creates a boson at the site $i$, $n_i = b_i^\dagger b_i$ is the number operator, and $\mu_i = \mu - \gamma R_{i,0}^2$ is the local chemical potential. The central chemical potential, $\mu$, tunes the average density, $\gamma$ parameterizes the parabolic confinement potential, and $R_{i,0} \equiv |\mathbf{R}_i - \mathbf{R}_0|$ is the distance between a site at $\mathbf{R}_i$ and the center of the trap, $\mathbf{R}_0$.

The mean field limit results from decoupled sites [5]:

$$-t \sum_{\langle i,j \rangle} (b_i^\dagger b_j + H.c.) \rightarrow -t \sum_{\langle i,j \rangle} \left( \psi_i^* b_j + b_i^\dagger \psi_j \right), \tag{7}$$

where $\psi_i \equiv \langle b_i \rangle$ is the local mean-field superfluid order parameter. The decoupling can be derived in an equivalent Gutzwiller formalism derived from a product variational wavefunction, where the variational amplitudes on each site can be shown to be directly related to $\psi_i$ [4, 6]. Using either (equivalent) formalism, the mean-field equations perform exceptionally well in 3D cubic lattices where quantum fluctuations are not as low as, say, in one dimension [7–14]. The local form of the mean-field equations allows us to simultaneously incorporate the spatial variations due to disorder (captured by spatial fluctuations in $\mu_i$ [15]) and spatial variations due to the trap. As such, these mean field equations capture the MI, SF, BG, and normal phases of the equilibrium Bose-Hubbard model in a trap.

The mean field equations further simplify in an extreme regime. In the absence of a finite SF density, we can take $\psi_i = \psi_i^* = 0$. This limit arises deep in the MI regime, ($t \ll U$), or at high temperatures, ($t \ll T$). Both limits are satisfied by the experiments discussed here; specifically we have $t \ll T \ll U$. We may therefore consider the much simpler atomic limit as a reasonable approximation:

$$H^A = \frac{U}{2} \sum_i n_i (n_i - 1) - \sum_i \mu_i n_i, \tag{8}$$

obtained by dropping the hopping term in Ref. 6 (this is the same as Eq. 1, but substitutes $\mu_i$ for the on site energy and trapping potential terms). The atomic limit captures compressible to incompressible transitions, as long as $t \ll T \ll U$. This regime therefore offers an excellent test bed for observations of compressibility.

In the regimes studied in this work (entropies per particle $\sim 0.8k_B - 1.2k_B$ and $t/U \lesssim 0.012$), we find $H^A$ to be an excellent approximation. We have compared all correlation functions we observe here using the atomic limit, Gutzwiller mean field theory, and quantum Monte Carlo. All methods agree in the parameter regimes studied. The quantum Monte Carlo method used, the stochastic series expansion with non-local updating [16, 17], is essentially exact. We conclude that the high dimensionality, high temperatures, and weak hopping all strongly suppress quantum fluctuations thus allowing $H^A$ to be used in direct comparison with experiment.

### B. Core Compressiblity

At zero temperature the Bose-Hubbard model supports an incompressible MI phase. The compressibility is given by:

$$\kappa = \frac{\partial \langle n \rangle}{\partial \mu}, \tag{9}$$

where $\langle n \rangle = N_s^{-1} \langle \sum_{i=1}^{N_s} n_i \rangle$ and $N_s$ is the total number of sites. Angular brackets denote the thermal average of observables: $\langle A \rangle = \mathrm{Tr}\left\{ A e^{-\beta H} \right\} / Z$, where $Z$ is the grand canonical partition function, $Z = \mathrm{Tr}\left\{ e^{-\beta H} \right\}$, and Tr denotes the trace. $\beta = (k_B T)^{-1}$ denotes the inverse temperature.

The compressibility allows us to track transitions from an incompressible MI phase to the BG as disorder is increased. The harmonic trap renders the entire system compressible (due to the existence of compressible edges), but the local compressibility can be used to examine incompressible regions. Once can show [18] that the local compressibility $\kappa_i$ is related to local particle number fluctuations: $\kappa_i = \beta \langle \Delta n_i^2 \rangle$, where

$$\langle \Delta n_i^2 \rangle \equiv \left\langle n_i^2 \right\rangle - \langle n_i \rangle^2 \tag{10}$$

Density fluctuations can be used to identify MI regions in a trap, because the MI gap suppresses fluctuations.

In the limit studied here, $t \ll T \ll U$, the MI state is nearly incompressible (the compressibility vanishes exponentially as $T$ shrinks with the energy scale set by the gap), whereas all other phases are compressible. Increasing disorder applied to a trapped MI at finite temperature then shows a transition from a (nearly) incompressible phase to a compressible phase.

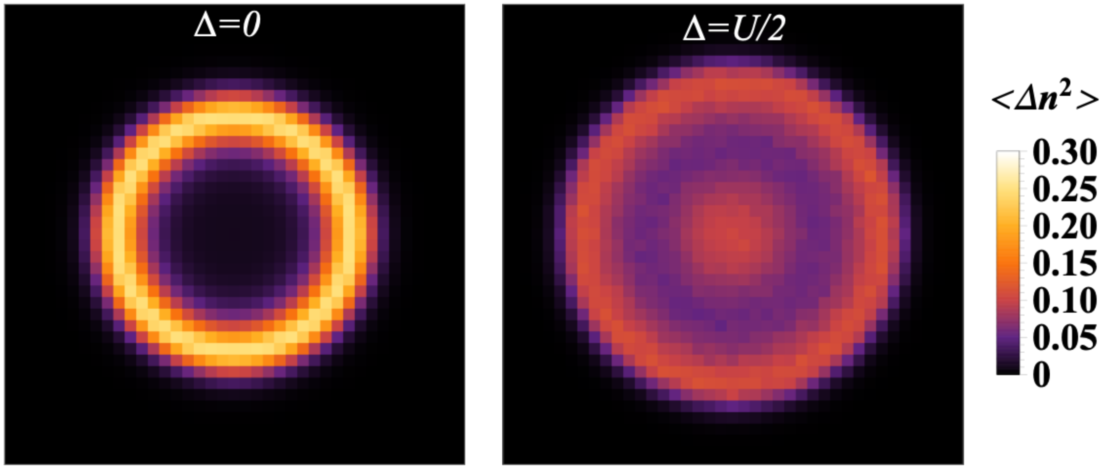


FIG. 6. Plot of the density fluctuations (Eq. 10) plotted in the $x-y$ plane of a 2D trapped lattice. The density fluctuations were obtained by using the Gutzwiller approximation to solve Eq. 6 with $U = 0.52E_R$, $\Omega^2 d^2/U = 4.7 \times 10^{-3}$, and $T = 20t = 0.096U$. The results were disorder averaged over 1000 realizations. The left panel, at $\Delta = 0$, shows essentially no density fluctuations near the trap center, consistent with the MI state. The right panel adds enough disorder, $\Delta = U/2$, to drive the center of the system into the compressible regime. The total compressibility is large and nearly the same for both panels because the system edges remain compressible.

Fig. 6 shows a plot of density fluctuations for a trapped MI for two different disorder strengths. The left panel shows that at zero disorder we see very little particle number fluctuations (dark region in the trap center), i.e., a nearly incompressible phase. The right panel shows that, for large disorder, we see particle number fluctuations in the trap center, and therefore a compressible phase. We therefore see that there is a transition captured by the local compressibility near the trap center.

The transition near the trap center can be measured with double occupancies [18–20]. The core compressibility ratio $\kappa_c^d/\kappa$ is given by [18]:

$$\frac{\kappa_c^d}{\kappa} = \frac{\partial \langle D \rangle}{\partial \mu} \left( \frac{\partial \langle N \rangle}{\partial \mu} \right)^{-1} \approx \frac{\partial \langle D \rangle}{\partial \langle N \rangle}. \tag{11}$$

The ratio $\kappa_c^d/\kappa$ is defined in terms of the core compressibility $\kappa_c^d$ (compressibility defined in terms of double occupancies) and the total compressibility, $\kappa$. The ratio on the right side, $\partial \langle D \rangle / \partial \langle N \rangle$, is a dimensionless quantity defined entirely in terms of optical lattice observables because the total number of particles, $\langle N \rangle = N_s \langle n \rangle$, and the total double occupancy, $D$, are both accessible from time of flight measurements. The total boson double occupancy is given by:

$$\langle D \rangle \equiv \left\langle \sum_i^{N_s} n_i \left( n_i - 1 \right) \right\rangle . \tag{12}$$

and is appreciable only near the core of the trapped system near the $\langle n \rangle = 1$ Mott lobe. Measurements of the slope of $\langle D \rangle$ vs. $\langle N \rangle$ therefore approximate the core compressibility.

We find that the total compressibility of the trapped system does not vary appreciably with disorder strength. For example, for $s = 20E_R$ we have $U = 0.52E_R$ and $t/U = 4.8 \times 10^{-3}$. For a trap frequency $\Omega^2 d^2/U = 4.7 \times 10^{-3}$ ($d = \lambda_{Lattice}/2 = 406$ nm is the lattice spacing) and entropy per particle $0.85k_{\mathrm{B}}$, we use $H^A$ to fit the double occupancy measured experimentally. The resulting total comprehensibility $\kappa$ of the trapped system increases by less than 7% as $\Delta$ is increased from 0 to 0.3 $E_R$ as we keep entropy fixed. We have tested other values of $s$ and find similar results indicating that the trap edges keep the comprehensibility nearly constant as we vary disorder for the parameters studied in this work. This allows us to conclude that measures of $\kappa_c^d/\kappa$ versus disorder strength effectively track changes in just $\kappa_c^d$.

### C. Incompressible-Compressible Transition in the Atomic Limit

We derive a simple expression for the disorder-driven incompressible-to-compressible transition in the atomic limit. We consider a single site with at most two bosons. The Hubbard model partition function becomes:

$$Z = 1 + \exp[\beta\mu] + \exp[\beta(2\mu - U)] \tag{13}$$

Using this partition function, we can derive the total compressibility as a function of chemical potential $\kappa(\mu)$ (from Eq. 9). The disorder average is obtained by integrating over the disorder distribution function$\mathcal{P}(\delta\mu)$:

$$\langle \kappa \rangle_{\mathrm{D}}(\mu_0) = \int_{-\Delta_{\min}}^{\Delta_{\max}} \kappa(\mu_0 + \delta\mu)\mathcal{P}(\delta\mu) d\delta\mu, \tag{14}$$

where the notation $\langle ... \rangle_{\rm D}$ indicates disorder averaging.

Assuming box disorder allows the derivation of a simple expression. For box disorder we have $\mathcal{P}_{\rm U}(\delta\mu) = 1/\Delta$, with $\Delta_{\rm min} = \Delta_{\rm max} = \Delta/2$. Near unity filling we set $\mu_0 = U/2$ and find:

$$\langle \kappa \rangle_{\rm D}(U/2) = \frac{2\left(e^{\beta\Delta} - 1\right)}{e^{\beta\Delta} + e^{\frac{1}{2}\beta(\Delta+U)} + 1}. \tag{15}$$

At temperatures well below $U$ this function becomes approximately $(2/\Delta)(1 + \exp[\beta(U - \Delta)/2])^{-1}$, with a form similar to a Fermi-Dirac distribution function. As such, the disorder averaged compressibility increases from zero as a step-like function of $\Delta$. The step near $\Delta = U$ indicates an incompressible to compressible transition. For temperatures near $U$ the step smooths out. Eq. 15 shows that the atomic limit allows the simplest example of a transition from an incompressible to a compressible regime driven by disorder. Here the transition energy is set by the Mott gap, $U$.

We find a similar transition for the exponential disorder distribution approximation to the speckle disorder applied in experiment, $\mathcal{P}_{\rm e}(\delta\mu) = \exp[-\delta\mu/\Delta]/\Delta$, with $\Delta_{\rm min} = 0$ and $\Delta_{\rm max} = \infty$. Here we note that the exponential distribution biases the chemical potential with increasing $\Delta$. To maintain near unity filling, we set the chemical potential to be $\mu = U/2 + \Delta$. Fig. 7 plots the core compressibility as a function of disorder obtained from Eq. 14 in the atomic limit without a trap. Here we fix entropy and observe that as we lower entropy, a sharp transition appears at $\Delta = U/2$. The entropy needs to be very low to see the sharp transition due to adiabatic heating with disorder. Therefore we do not expect to see the sharp transition in the measurements presented here.

### D. Atomic Limit Threshold Disorder and Comparison to Experiment

To compare to experimental data, a prediction of $D$ and $N$ is obtained in the atomic limit using the same parameters as the experiment—including the harmonic trap (adding disorder to the calculation presented in section I C). A small area around the center of the trap was sampled ($\mu = 0.5 + \Delta \pm 0.02$) to determine the core compressibility. The relationship between $D$ and $N$ at unit filling is determined by averaging over 100 disorder realizations and extracting the slope.

The experimental $\partial D/\partial N$ data is analyzed using least-squares fitting with a discontinuous, piecewise linear function where the threshold disorder, the disorder strength at which

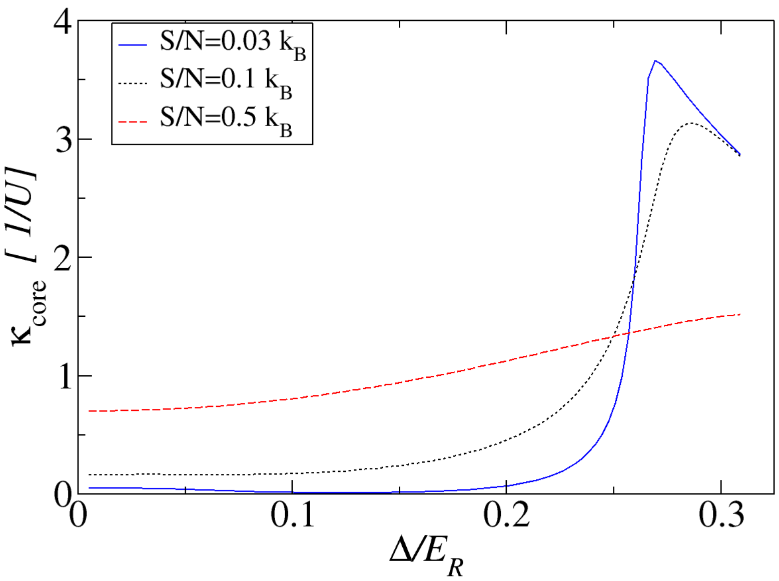


FIG. 7. Plot of the core compressibility, $\partial \langle D \rangle / \partial \mu$, as function of disorder computed using Eq. 14 in the atomic limit at fixed entropy. This calculation is for a uniform system. Three entropies are chosen to show that at low entropy, exponentially distributed disorder leads to a transition from a (nearly) incompressible MI phase to a compressible phase near $\Delta = U/2$. We set $U = 0.52E_R$ to make contact with the interaction energy scale in experiments at $s = 20$.

the slope changes, is used as a simple metric for agreement with theory. Analysis of the data using a fitting function characteristic of zero temperature behavior is motivated by technical reasons. Employing a continuous fitting function results in large uncertainties in the fitting parameters. This occurs because of the scatter and uncertainty in the data points and the larger number of fitting parameters needed to specify the continuous fitting function. Furthermore, the amount of scatter makes it difficult to distinguish continuous and discontinuous compressibility behavior. Practically, this limitation means it is only possible to determine when the compressibility rises above the scatter in the baseline value at low disorder, providing further motivation for using the piecewise linear function.

In order to establish that the piecewise analysis is a suitable method for making quantitative comparison between experiment and theory, it is necessary to show that the threshold disorder is appropriately sensitive to entropy-per-particle $S/N$. For small $\Delta$, theory predicts that the baseline compressibility level is set by $S/N$, as shown in Fig. 8, and remains nearly constant for a range of $\Delta$ which becomes progressively smaller as $S/N$ increases. Similarly,

| $s$ ($E_R$) | $U/2$ ($E_R$) | $\Delta_{th}^{AL}(S/N=0)$ ($E_R$) |
|---|---|---|
| 16 | 0.22 | $0.27 \pm 0.01$ |
| 20 | 0.26 | $0.29 \pm 0.01$ |
| 25 | 0.32 | $0.34 \pm 0.02$ |

TABLE II. Comparison of the threshold disorder predicted in the atomic limit, $\Delta_{th}^{AL}$ at $S/N = 0$ to $U/2$ for each of the lattice strengths measured.

the threshold disorder should decrease with increasing $S/N$. To make an accurate and fair comparison between experiment and theory, the noise characteristics of the experimental data must be combined with the theory. This is accomplished by sampling the predicted compressibility according to the uncertainty in $\partial D/\partial N$ to obtain simulated data at each $S/N$. The simulated data is fit using the piecewise linear function, and the threshold disorder is averaged over 100 realizations to obtain the sampling threshold disorder, $\Delta_{th}^{s}$. The desired behavior of $\Delta_{th}^{s}$ vs $S/N$ is found as demonstrated in Fig. 9 for $s/E_R = 16$, validating the use of this analysis method in the experiment. As a consistency check, $\Delta_{th}^{AL}(S/N = 0)$ is compared to $U/2$ in Table II. Good agreement is found for $s/E_R = 20$ and 25, but not for $s/E_R = 16$. The theory neglects tunneling, which is stronger for lower lattice depths and may explain the discrepancy for $s/E_R = 16$. The linear fit in Fig. 9 is used to find the predicted threshold disorder at the $S/N$ of the experiment. The uncertainty comes from the product of the uncertainty in $S/N_{average}$ and the slope of the line of best fit to $\Delta_{th}^{AL}$ vs $S/N$.

### E. Energy Gap and Inverse Compressibility

The inverse compressibility can be directly related to the Mott-state energy gap at zero temperature. In a closed, finite sized-system, we define the energy gap, $\delta\mu$, as sum of the energy to add a single particle to the $N$-particle system ($E_{N+1} - E_N$)and the energy to subtract a particle ($E_{N-1} - E_N$):

$$\delta\mu = E_{N+1} + E_{N-1} - 2E_N. \tag{16}$$

From this expression we see that, for a system where the particle number can vary by a non-integer, $\delta\langle n\rangle$, the energy gap per particle becomes $\delta\mu/\delta\langle n\rangle$, which is the inverse compressibility in the thermodynamic limit. Another way to see the connection between the

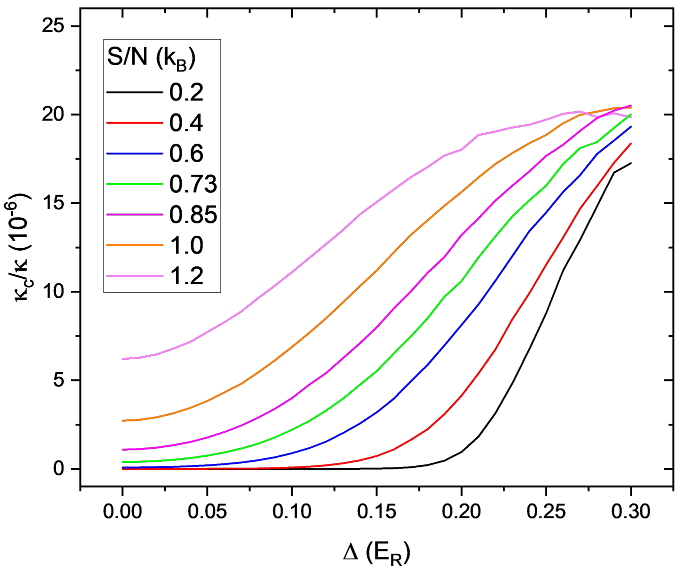


FIG. 8. Atomic limit prediction for the core compressibility ratio at $s/E_R = 16$ as a function of $S/N$. The curves are generated at example values of $S/N$. The fractional uncertainty is less than 1%. The calculation used the same parameters as the trap, including the harmonic trap. To obtain the core compressibility, the chemical potential was varied to select a small region around the trap center (from $\mu = 0.5 + \Delta - 0.02$ to $\mu = 0.5 + \Delta + 0.02$). A sample of 31 points was used to obtain the relationship between $D$ and $N$. The slope was calculated by averaging 100 disorder realizations.

energy gap and the inverse compressibility is to note that $E_{N+1} + E_{N-1} - 2E_N$ is the discrete second derivative of the total energy with respect to particle number. The second derivative of the total energy with respect to total energy is proportional to the inverse compressibility.

The non-zero gap inferred from the inverse compressibility can be used to track closing of the gap. Finite temperature includes others states. The inverse compressibility then signals a true gap as temperature is taken to zero. Nonetheless, for temperatures much lower than the gap, we can say that with increasing disorder the gap shrinks and the system becomes more compressible. Fig. 10 plots the inverse compressibility as function of average chemical potential. Peaks correspond to chemical potentials with non-zero gaps (the center of the MI regime).

We have checked that the core compressibility shows analogous peaks. We have also checked that exponential disorder leads to similar behavior. We conclude that the inverse

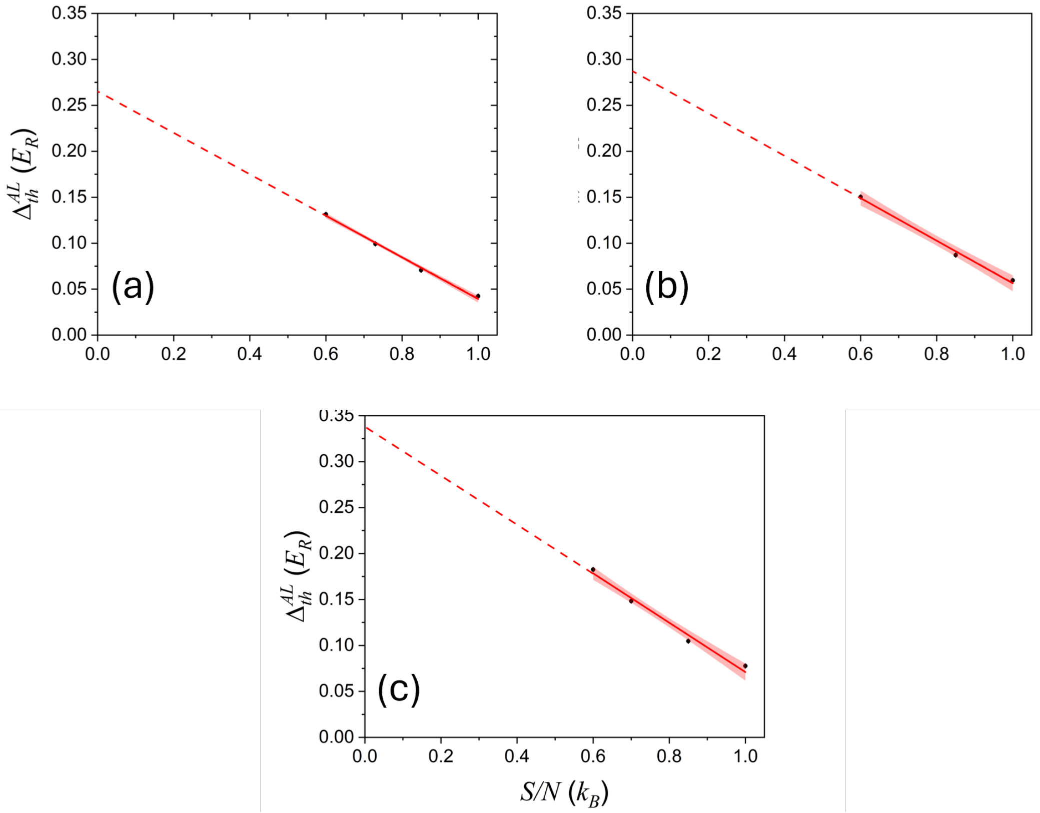


FIG. 9. Threshold disorder obtained from sampling theory at different $S/N$ for lattice depths $s = 16$ (a), $s = 20$ (b), and $s = 25$ (c). The black points and their uncertainty are obtained from averaging 5 sampling realizations. The red line is a linear fit to the black points and the red shaded region is the 68% confidence band. Comparison to experiment is done using the results of the linear fit.

core compressibility can be used to measure the closing of the gap as disorder is increased. This connection is reasonable at non-zero temperature provided the temperature is much lower than the energy gap.

### F. Adiabatic Heating by Disorder

Increasing disorder adiabatically leads to higher temperatures [21]. We can understand adiabatic heating in the micro-canonical ensemble. Increasing disorder in the single-band Hubbard model decreases the number of available sites which would otherwise lower entropy because the entropy scales with the log of the number of available configurations. But at fixed entropy the system must populate excited states, i.e., raise its temperature, to maintain a

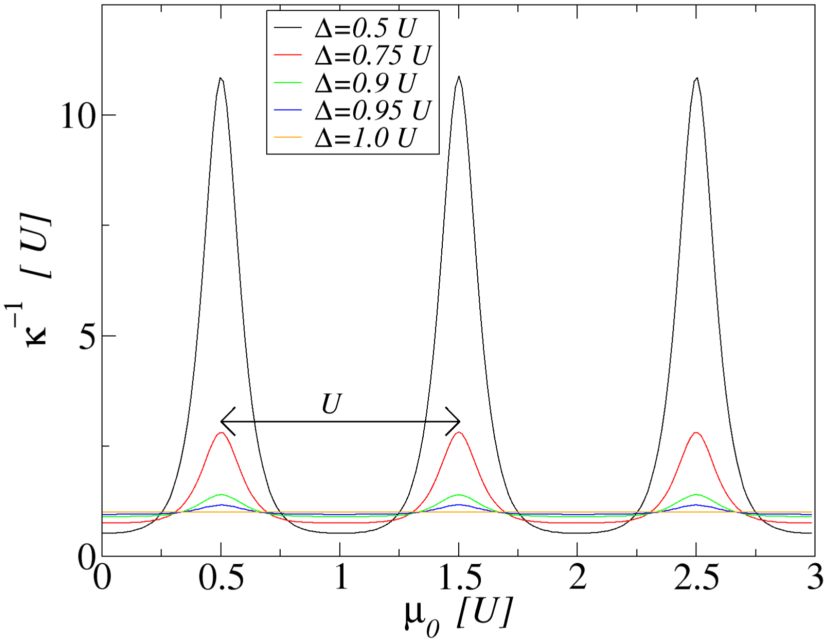


FIG. 10. Plot of the inverse compressibility as a function of the average compressibility computed in the atomic limit for box disorder of strength $\Delta$ for fixed temperature $T = U/15$. At zero temperature and zero disorder, peaks in the inverse compressibility show the energy spacing between different MIs. The horizontal line labels the spacing $U$ between the $\langle n \rangle = 1$ and $\langle n \rangle = 2$ MIs. Increasing temperature and disorder broadens the peaks. Above a critical disorder strength, $\Delta = U$, the different Mott regimes cannot be resolved.

fixed entropy. Increasing disorder at fixed entropy therefore also increases temperature [21]. We conclude that the incompressible-to-compressible transition studied here is a thermal transition as well as a transition induced by disorder.

We estimate the impact of adiabatic heating in our simulations. Fig. 11 shows results from the atomic limit plotting temperature as function of disorder at *fixed entropy* for parameters consistent with experiments. We find that the temperature increases from $19t/k_B$ to $27t/k_B$ as we increase $\Delta$ from 0 to 0.3 $E_R$, where we choose parameters for $s = 20E_R$ ($U = 0.52E_R$ and $t/U = 4.8 \times 10^{-3}$) with a trap frequency $\Omega^2 d^2/U = 4.7 \times 10^{-3}$ and entropy per particle $0.85k_{\mathrm{B}}$. This shows that fixing entropy forces the temperature to increase appreciably as we increase disorder strength (i.e., adiabatic heating by disorder). The increase in disorder therefore further suppresses the impact of quantum fluctuations (by increasing thermal fluctuations) leaving $H^A$ as an even better approximation to $H$. As a check on the regime $t \ll k_B T \ll U$, Table III shows the temperature for each lattice depth across the

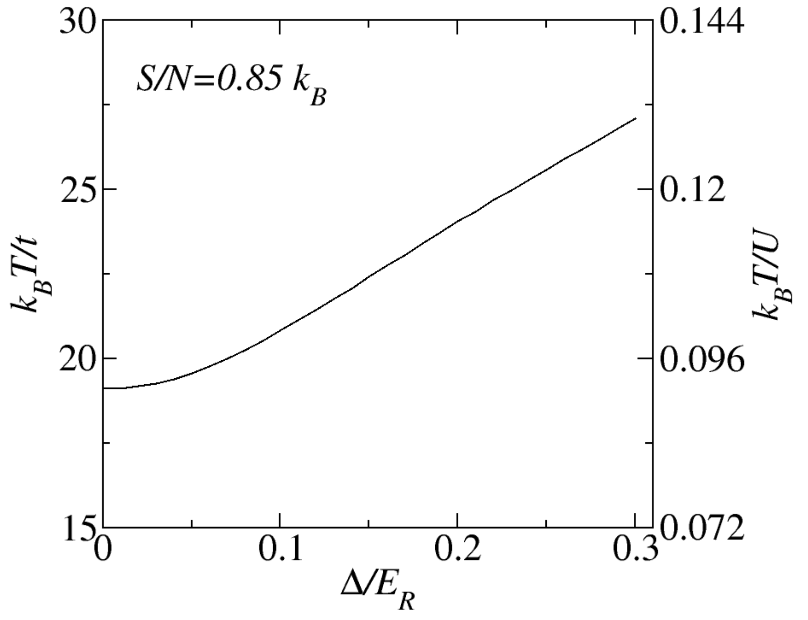


FIG. 11. Temperature of the trapped system as a function of disorder strength at a representative fixed entropy per particle, $S/N = 0.85k_{\rm B}$, computed using disorder averaging of exponentially distrubted disorder in the atomic limit. The parameters are chosen to match $s = 20$ experimental parameters with $U = 0.52E_{\rm R}$, $\gamma/U = 4.7 \times 10^{-3}$, and $\mu_0 = U/2 + \Delta$. The plot shows adiabatic heating resulting from increased disorder.

| $s(E_R)$ | $t/U$ | $k_BT/U$ $(\Delta = 0)$ | $k_BT/U$ $(\Delta_{th}^{exp})$ | $k_BT/U$ $(\Delta_{max})$ |
|---|---|---|---|---|
| 16 | 0.0124 | 0.0745 | 0.0791 | 0.1001 |
| 20 | 0.0048 | 0.0882 | 0.1017 | 0.1132 |
| 25 | 0.0017 | 0.0746 | 0.0841 | 0.1016 |

TABLE III. Tunneling energy and calculated temperatures at various $\Delta$ for each lattice depth $s$. Three representative disorder strengths are chosen: the clean lattice case $\Delta = 0$, the experimentally measured threshold disorder for each lattice depth $\Delta_{th}^{exp}$, and the maximum disorder strength realized $\Delta_{max}$. The temperatures are calculated based on the $S/N$ values determined by measurements at $\Delta = 0$. For all disorder strengths the temperature is in the regime $t \ll k_BT \ll U$.

range of disorders realized in the experiment.

The increase in temperature forces the system to miss the BG regime. If we assume that the system is in thermal equilibrium is as we increase disorder, we find temperature

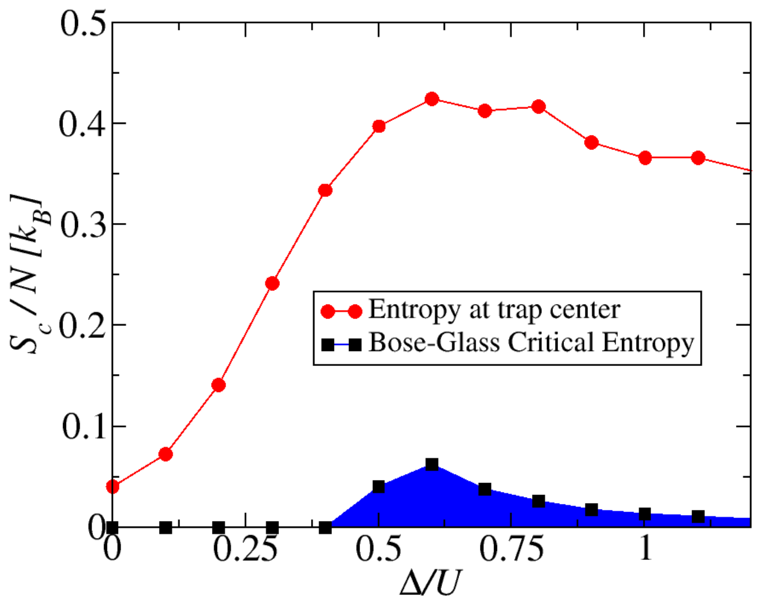


FIG. 12. The circles plot the entropy at the center of the trap as function of disorder computed for parameters chosen to match $s = 20$ experimental parameters with $U = 0.52E_{\mathrm{R}}$, $\gamma/U = 4.7 \times 10^{-3}$, and $\mu_0 = U/2$. The total entropy per particle is fixed to $0.8k_{\mathrm{B}}$. The increase in the entropy at the center arises from a redistribution of thermal fluctuations within the trap as disorder overcomes the Mott gap. The squares plot the upper bound on the entropy needed to achieve a BG computed for the same parameters but in a system with no trap using Gutzwiller mean-field theory. Comparing both data sets shows that entropy near the center of the trap is too high to reach the BG regime.

that are much higher than the BG transition temperature. The left $y$-axis of Fig. 12 plots the critical entropy needed to observe the BG a uniform system at lattice depth $s = 20$, i.e., the Bose-Hubbard model with $t/U = 0.0048$ and no trap. Here we use the Gutzwiller approximation with the local fluctuations of particle number, $\langle b_i^\dagger \rangle$, as a bound on the local condensate fraction. The dome shows that as disorder increases, the MI gives way to a BG with a critical entropy per particle below 0.05 $k_{\mathrm{B}}$. The right $y$-axis plots the entropy at the center of the trap for the same parameters used in Fig. 6. The entropy at the center is well defined in the atomic limit. Here we see that even though the total entropy is fixed, local

heating near the trap center causes the effective entropy to increase.

---


[1] D. McKay and B. DeMarco, Thermometry with spin-dependent lattices, New J. Phys. **12**, 055013 (2010).

[2] A. Widera, F. Gerbier, S. Fölling, T. Gericke, O. Mandel, and I. Bloch, Coherent collisional spin dynamics in optical lattices, Phys. Rev. Lett. **95**, 190405 (2005).

[3] A. Widera, F. Gerbier, S. Fölling, T. Gericke, O. Mandel, and I. Bloch, Precision measurement of spin-dependent interaction strengths for spin-1 and spin-2 $^{87}$Rb atoms, New J. Phys. **8**, 152 (2006).

[4] D. Jaksch, C. Bruder, J. I. Cirac, C. W. Gardiner, and P. Zoller, Cold Bosonic Atoms in Optical Lattices, Phys. Rev. Lett. **81**, 3108 (1998).

[5] S. Sachdev, *Quantum Phase Transitions* (Cambridge University Press, 2000).

[6] D. S. Rokhsar and B. G. Kotliar, Gutzwiller projection for bosons, Phys. Rev. B **44**, 10328 (1991).

[7] J. Zakrzewski, Mean-field dynamics of the superfluid-insulator phase transition in a gas of ultracold atoms, Phys. Rev. A **71**, 043601 (2005).

[8] K. Sheshadri, H. R. Krishnamurthy, R. Pandit, and T. V. Ramakrishnan, Percolation-Enhanced Localization in the Disordered Bosonic Hubbard Model, Phys. Rev. Lett. **75**, 4075 (1995).

[9] B. Damski, J. Zakrzewski, L. Santos, P. Zoller, and M. Lewenstein, Atomic Bose and Anderson Glasses in Optical Lattices, Phys. Rev. Lett. **91**, 080403 (2003).

[10] P. Buonsante, V. Penna, A. Vezzani, and P. B. Blakie, Mean-field phase diagram of cold lattice bosons in disordered potentials, Phys. Rev. A **76**, 011602 (2007).

[11] P. Buonsante, F. Massel, V. Penna, and A. Vezzani, Gutzwiller approach to the bose-hubbard model with random local impurities, Phys. Rev. A **79**, 013623 (2009).

[12] I. Hen and M. Rigol, Superfluid to Mott insulator transition of hardcore bosons in a superlattice, Phys. Rev. B **80**, 134508 (2009).

[13] I. Hen and M. Rigol, Analytical and numerical study of trapped strongly correlated bosons in two- and three-dimensional lattices, Phys. Rev. A **82**, 043634 (2010).

[14] N. Lin, E. Gull, and A. J. Millis, Two-particle response in cluster dynamical mean-field theory:

Formalism and application to the raman response of high-temperature superconductors, Phys. Rev. Lett. **109**, 106401 (2012).

[15] S. Q. Zhou and D. M. Ceperley, Construction of localized wave functions for a disordered optical lattice and analysis of the resulting Hubbard model parameters, Phys. Rev. A **81**, 013402 (2010).

[16] B. Bauer, L. D. Carr, H. G. Evertz, A. Feiguin, J. Freire, S. Fuchs, L. Gamper, J. Gukelberger, E. Gull, S. Guertler, A. Hehn, R. Igarashi, S. V. Isakov, D. Koop, P. N. Ma, P. Mates, H. Matsuo, O. Parcollet, G. Pawłowski, J. D. Picon, L. Pollet, E. Santos, V. W. Scarola, U. Schollwöck, C. Silva, B. Surer, S. Todo, S. Trebst, M. Troyer, M. L. Wall, P. Werner, and S. Wessel, The alps project release 2.0: open source software for strongly correlated systems, J. Stat. Mech.: Theor. Exp. **2011**, P05001 (2011).

[17] A. W. Sandvik, Stochastic series expansion method with operator-loop update, Phys. Rev. B **59**, 157 (1999).

[18] Y. Khorramzadeh, F. Lin, and V. W. Scarola, Boson core compressibility, Phys. Rev. A **85**, 043610 (2012).

[19] R. Jördens, N. Strohmaier, K. Günter, H. Moritz, and T. Esslinger, A Mott insulator of fermionic atoms in an optical lattice, Nature (London) **455**, 204 (2008).

[20] V. W. Scarola, L. Pollet, J. Oitmaa, and M. Troyer, Discerning incompressible and compressible phases of cold atoms in optical lattices, Phys. Rev. Lett. **102**, 135302 (2009).

[21] V. W. Scarola and B. DeMarco, Dynamics of Hubbard-band quasiparticles in disordered optical lattices, Phys. Rev. A **92**, 053628 (2015).
